# Supplementary material for: Learning Deep Features in Instrumental Variable Regression
Source: arXiv:2010.07154 source file (2023-06-27)
Supplement: Supplementary file 1 [file feature_map_learning.tex]

Here, we compare the approach of learning the adaptive feature maps to the learning of an ordinary feedforward network. Let consider the following regression problem:
\begin{align*}
    \hat{\vec{u}}, \hat{\theta} = \argmin_{\vec{u}, \theta} \mathcal{L}(\vec{u}, \theta), \quad \mathcal{L}(\vec{u}, \theta)=\frac{1}{n} \sum_{i=1}^n \|y_i - \vec{u}^\top \vec{\phi}_\theta(x_i)\|^2 + \lambda\|\vec{u}\|^2,
\end{align*}
where $(x_i, y_i)$ are data, and $\vec{\phi}_\theta$ denotes the adaptive feature map parameterized by $\theta$. If we use a simple feedforward neural network, this is learned by jointly updating $\vec{u}$ and $\theta$ using gradient descent methods:
\begin{align*}
    \hat{\vec{u}}_{t+1} \leftarrow \hat{\vec{u}}_{t} - \nabla_{\vec{u}}  \mathcal{L}(\vec{u}, \hat{\theta}_t)|_{\vec{u}=\hat{\vec{u}}_{t}}, \quad \hat{\theta}_{t+1} \leftarrow \hat{\theta}_{t} - \nabla_{\theta}  \mathcal{L}(\hat{\vec{u}}_t, \theta)|_{\theta=\hat{\theta}_{t}},
\end{align*}
where $\hat{\vec{u}}_t$ and $\hat{\theta}_t$ are the estimates of $\vec{u}$ and $\theta$ at the $t$-th epoch, respectively.
We refer to this approach as {\tt Joint-Gradient-Descent}. The approach we used is to first solve the minimization problem to get $\hat{\vec{u}}$ fixing $\theta$. We have indeed:
\begin{align*}
    \hat{\vec{u}}(\theta)&:= \argmin_{\vec{u}} \mathcal{L}(\vec{u}, \theta)=\left(\Phi_t^\top \Phi_t + n \lambda I\right)^{-1}\left(\Phi_t^\top \vec{y}\right),
\end{align*}
where $\Phi_t = [\vec{\phi}_{\theta}(x_1), \dots, \vec{\phi}_{\theta}(x_n)]^\top$ and  $\vec{y} = [y_1, \dots, y_n]^\top$. 
Then, we set:
\begin{align*}
    \hat{\vec{u}}_{t+1} \leftarrow \hat{\vec{u}}(\hat{\theta}_t), \quad 
    \hat{\theta}_{t+1} \leftarrow \hat{\theta}_{t} - \nabla_{\theta}\mathcal{L}(\hat{\vec{u}}(\theta),\theta)|_{\theta=\hat{\theta}_t}.
\end{align*}
%\begin{align*}
%    \hat{\vec{u}}_{t+1} \leftarrow \left(\Phi_t^\top \Phi_t + n \lambda I\right)^{-1}\left(\Phi_t^\top \vec{y}\right), \quad 
%    \hat{\theta}_{t+1} \leftarrow \hat{\theta}_{t} - \nabla_{\theta}\mathcal{L}(\hat{\vec{u}}_{t+1},\theta),
%\end{align*}
%where $\Phi_t = [\vec{\phi}_{\hat{\theta}_t}(x_1), \dots, \vec{\phi}_{\hat{\theta}_t}(x_n)]^\top$ and  $\vec{y} %= [y_1, \dots, y_n]^\top$. 
We call this approach {\tt Feature-Map-Learning}. 

Here, we empirically compare the {\tt Joint-Gradient-Descent} and {\tt Feature-Map-Learning} approaches. We used a 3-layer fully connected neural nets as $\vec{\phi}_\theta$, where it maps input $x$ to a 32-dimensional vector. The size of the hidden layer is set to 64. We used the MNIST dataset, where $x_i$ is the image and $y_i$ is the label, and ADAM for gradient-based optimization. Figure~\ref{fig:feature_map_learning} shows the learning curves of the two approaches. From Figure~\ref{fig:feature_map_learning}, we can see that {\tt Feature-Map-Learning} converges faster than {\tt Joint-Gradient-Descent} and reaches a solution that generalizes well.

\begin{figure}
    \begin{small}
        \begin{center}
            \includegraphics[width=0.95\textwidth]{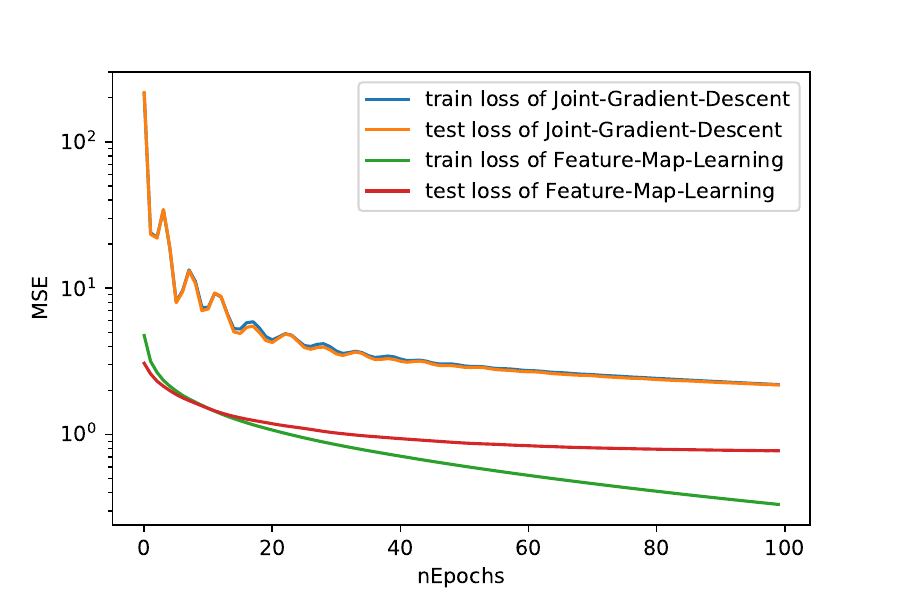}
        \end{center}
        \caption{Comparison of two approaches}
        \label{fig:feature_map_learning}
    \end{small}
\end{figure}
