# Supplementary material for: Learning Deep Features in Instrumental Variable Regression
Source: arXiv:2010.07154 source file (2023-06-27)
Supplement: Supplementary file 2 [file test_points.tex]

Figure~\ref{fig:testpoints} shows plot of $(p,t)$ appears in train time and test time.
the train points and test points in the demand design problem. From Figure~\ref{fig:testpoints}, we can see that the model is required to predict the points where no training point exists. In other words, the model needs to extrapolate the prediction in order to achieve a good performance in this experiment.

\begin{figure}[H]
    \begin{small}
        \begin{center}
            \includegraphics[width=0.7\textwidth]{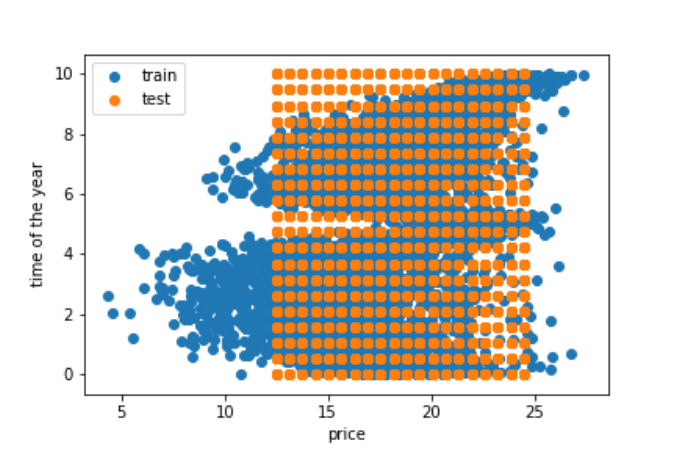}
        \end{center}
        \caption{train points and test points of price $p$ and time of the year $t$}
        \label{fig:testpoints}
    \end{small}
\end{figure}

Such change of distribution damages the vanilla DFIV, which Spectral Normalization is not applied. Figure~\ref{fig:fail} shows the 200 test points with the largest prediction error.

\begin{figure}[H]
    \begin{small}
        \begin{center}
            \includegraphics[width=0.7\textwidth]{Appendix/failing.pdf}
        \end{center}
        \caption{200 test points that vanilla DFIV fails}
        \label{fig:fail}
    \end{small}
\end{figure}

From Figure~\ref{fig:fail}, we can see that the vanilla DFIV fails at the test points where there is little training points around.
To deal with this problem, we need to make have to impose smoothness on the model we learn. This is the reason why this setting is favorable for KIV\citep{Singh2019} method, which uses the prespecified smooth feature maps. DeepIV\citep{Hartford2017} also implicitly regularizes the model by stochastically perturbing the input to Stage 2 regression problem according to the conditional distribution estimated in Stage 1 regression.
