# Supplementary material for: Learning Deep Features in Instrumental Variable Regression
Source: arXiv:2010.07154 source file (2023-06-27)
Supplement: Supplementary file 4 [file proof-thm-1.tex]

Here, we prove Theorem~\ref{thm:approximation}, which states that our simple kernel function can express the complex function.

\begin{proof}
    Let $\kappa$ be a shift-invariant kernel function on $[0,1]^d$. From Claim 1 in \citet{Rahimi2008}, there exists a random algorithm that generates random matrix $A \in \mathbb{R}^{D\times d}$ and vector $\vec{b} \in \mathbb{D}$ such that
    \begin{align*}
        \prob{\sup_{\vec{x}, \vec{y}}\|(\cos(A\vec{x} + \vec{b}))^\top(\cos(A\vec{y} + \vec{b})) - \kappa(\vec{x}, \vec{y})\|^2 \geq \varepsilon} \leq 2^8 \frac{\sigma_p^2 d}{\varepsilon^2}\exp\left(-\frac{D\varepsilon^2}{4(d+2)}\right),
    \end{align*}
    where $\sigma_p$ is a constant depending on $\kappa$ and cosine function is appled element-wise $\cos(\vec{x}) = (\cos(x_1), \cos(x_2), \dots)^\top$. From the inequality above, we can see that the probability is strictly less than 1 if we set $D = \Omega(\frac{d}{\varepsilon^2}\log\frac{d}{\varepsilon})$. Hence, we can conclude that there exists $\tilde A, \tilde{\vec{b}}$ such that 
    \begin{align*}
        \sup_{\vec{x}, \vec{y}}\|(\cos(\tilde A\vec{x} + \tilde{\vec{b}}))^\top(\cos(\tilde A\vec{y} + \tilde{\vec{b}})) - \kappa(\vec{x}, \vec{y})\|^2 \leq \varepsilon
    \end{align*}
    from the probablistic method \citep{alon04}. Therefore, the $L+1$-layer network  $\tilde\psi(\vec{x}) = \cos(\tilde A\vec{x} + \tilde{\vec{b}})$ satisfies the condition given in the theorem.
\end{proof}
