# Supplementary material for: Learning Deep Features in Instrumental Variable Regression
Source: arXiv:2010.07154 source file (2023-06-27)
Supplement: Supplementary file 5 [file feature_map_learning.tex]

Here, we compare the approach of learning the adaptive feature maps to the learning the ordinary feed-forward network. Let consider the following regression problem.
\begin{align*}
    \hat{\vec{f}}, \hat{\theta} = \argmin_{\vec{f}, \theta} \mathcal{L}(\vec{f}, \theta), \quad \mathcal{L}(\vec{f}, \theta)= \sum_{i=1}^n \|y_i^2 - \vec{f}^\top \vec{\phi}_\theta(x_i)\|^2 + \lambda\|\vec{f}\|^2,
\end{align*}
where $(x_i, y_i)$ are data, and $\vec{\phi}_\theta$ denotes the adaptive feature map parmameterized by $\theta$. If we use simple feedforward neural network, this is learned by jointly update $\vec{f}$ and $\theta$ using gradient-decent methods.
\begin{align*}
    \hat{\vec{f}}_{t+1} \leftarrow \hat{\vec{f}}_{t} - \nabla_{\vec{f}}  \mathcal{L}(\vec{f}, \hat{\theta}_t), \quad \hat{\theta}_{t+1} \leftarrow \hat{\theta}_{t} - \nabla_{\theta}  \mathcal{L}(\hat{\vec{f}}_t, \theta),
\end{align*}
where $\hat{\vec{f}}_t$ and $\hat{\theta}_t$ are the estimation of $\hat{\vec{f}}$ and $\hat{\theta}$ at $t$-th epoch, respectively.
Let us call this approach as {\tt Joint-Gradient-Descent}. The approach we used is to first solve the minimization problem to get $\hat{\vec{f}}$ fixing $\theta$. Then, take a gradient step for $\vec{f} = \hat{\vec{f}}_t$.
\begin{align*}
    \hat{\vec{f}}_{t+1} \leftarrow \left(\Phi_t^\top \Phi_t + \lambda I\right)^{-1}\left(\Phi_t^\top \vec{y}\right), \quad 
    \hat{\theta}_{t+1} \leftarrow \hat{\theta}_{t} - \nabla_{\theta}\mathcal{L}(\hat{\vec{f}}_{t+1},\theta)
\end{align*}
where $\Phi_t = [\vec{\phi}_{\hat{\theta}_t}(x_1), \dots, \vec{\phi}_{\hat{\theta}_t}(x_n)]^\top$ and  $\vec{y} = [y_1, \dots, y_n]^\top$. Let us call this approach as {\tt Feature-Map-Learning}. 

Here, we empirically compare {\tt Joint-Gradient-Descent} approach and {\tt Feature-Map-Learning} approach. We used 3-layer fully connected neural nets as $\vec{\phi}_\theta$, where it maps input $x$ to 32-dimensional vector. The size of the hidden layer is set to 64. We used MNIST datasets, where $x_i$ is the image and $y_i$ is the label. We used ADAM for gradient-based optimization algorithm. Figure~\ref{fig:feature_map_learning} shows the learning curves of the two approaches. From Figure~\ref{fig:feature_map_learning}, we can see that {\tt Feature-Map-Learning} approach converges faster than {\tt Joint-Gradient-Descent} and reaches to the solution that generalizes well.

\begin{figure}
    \begin{small}
        \begin{center}
            \includegraphics[width=0.95\textwidth]{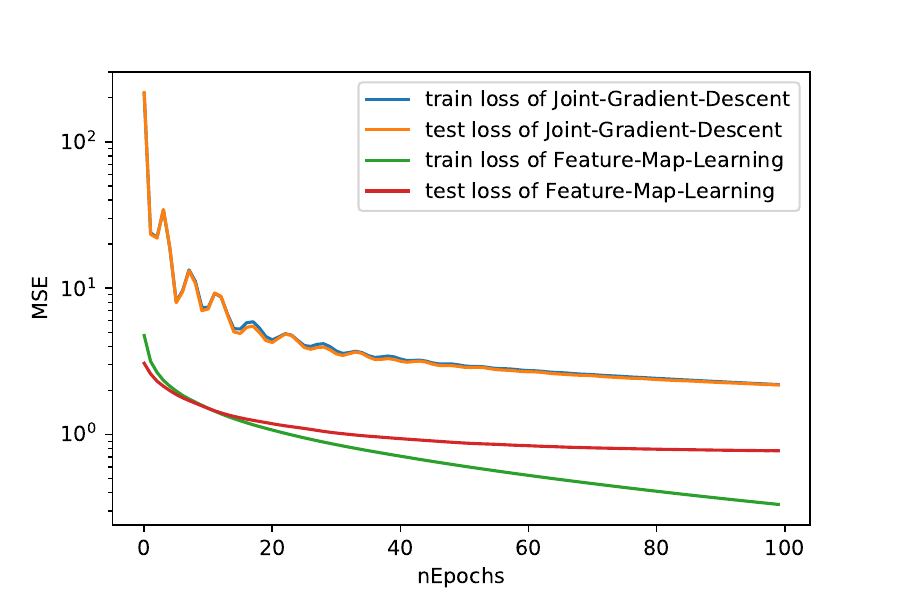}
        \end{center}
        \caption{Comparison of two approaches}
        \label{fig:feature_map_learning}
    \end{small}
\end{figure}
