# Supplementary material for: Learning Deep Features in Instrumental Variable Regression
Source: arXiv:2010.07154 source file (2023-06-27)
Supplement: Supplementary file 6 [file hyper-param.tex]

In this appendix, we introduce the way of tuning the hyper-parameter $\lambda_1, \lambda_2$. In KIV, this is done by optimizing the stage 1 and stage 2 error evaluated by the out-of-sample. This approach, however, is not valid in DFIV since we alternatively update stage 1 model and stage 2 model. Instead, we propose to choose hyper-parameter jointly from the out-of-sample stage 2 loss. Formally, let denote complete stage 1 data as $(x_i, y_i, z_i)$, and $\lambda_1, \lambda_2$ is chosen that minimizes
\begin{align*}
    \hat{\mathcal{L}}_2^{(\mathrm{oos})} = \frac{1}{m} \sum_{i=1}^m \|y_i - (\hat{\vec{f}}^{(n)})^\top \hat{E}^{(m)} \vec{\phi}_{\theta_Z}(z_i)\|^2.
\end{align*}
Note that $\hat{E}^{(m)}$ and $\hat{\vec{f}}^{(n)}$ are the solution of stage 1 and 2, respectively.
